# Supplementary material for: nocaps: novel object captioning at scale
Source: arXiv:1812.08658 source file (2019-09-30)
Supplement: Supplementary file 1 [file nbt_fg_table.tex]

\begin{table*}[h]
\begin{center}
\footnotesize
\begin{tabularx}{\textwidth}{ll}
\toprule
\textbf{Object class} & \textbf{Fine-grained class} \\
\midrule

\ttbf{airplane}         & \tt{jetliner, plane, air plane, monoplane, aircraft, jet, airbus, biplane, seaplane} \\

\ttbf{backpack}         & \tt{knapsack} \\

\ttbf{ball}             & \tt{sports ball, baseball, soccer, basketball, softball, pinball, fastball, racquetball} \\

\ttbf{bear}             & \tt{panda} \\

\ttbf{bench}            & \tt{pew} \\

\ttbf{bicycle}          & \tt{bike, minibike, trike} \\

\ttbf{bird}             & \tt{seagull, parakeet, robin, pelican, waterfowl, heron, hummingbird, mallard, finch, pigeon, seabird, osprey,} \\
                        & \tt{blackbird, fowl, shorebird, egret, chickadee, quail, bluebird, kingfisher, buzzard, willet, gull, bluejay,} \\
                        & \tt{flamingo, cormorant, loon, gosling, waterbird, pheasant, rooster, sandpiper, crow, oriole, cowbird,}        \\
                        & \tt{warbler, peacock, cockatiel, lorikeet, puffin, vulture, condor, macaw, peafowl, cockatoo, songbird}         \\

\ttbf{boat}             & \tt{ship, liner, sailboat, motorboat, dinghy, powerboat, speedboat, skiff, yacht, kayak, catamaran, pontoon,}   \\
                        & \tt{houseboat, vessel, rowboat, trawler, ferryboat, watercraft, tugboat, schooner, barge, ferry, sailboard,}    \\
                        & \tt{paddleboat, lifeboat, freighter, steamboat, riverboat, battleship, steamship, surfboard, longboard,}        \\
                        & \tt{skimboard, shortboard, wakeboard}                                                                           \\

\ttbf{cake}             & \tt{cheesecake, cupcake, shortcake, coffeecake} \\

\ttbf{car}              & \tt{automobile, van, minivan, sedan, suv, hatchback, cab, jeep, coupe, taxicab, limo, taxi} \\

\ttbf{cat}              & \tt{kitten, feline, tabby} \\

\ttbf{cattle}           & \tt{cow, oxen, ox, calf, ewe, holstein, heifer, buffalo, zebu, bison} \\

\ttbf{chair}            & \tt{seat, recliner, stool} \\

\ttbf{dog}              & \tt{puppy, beagle, pup, chihuahua, schnauzer, dachshund, rottweiler, canine, pitbull, collie, pug, terrier,}    \\
                        & \tt{poodle, labrador, doggie, doberman, mutt, doggy, spaniel, bulldog, sheepdog, weimaraner, corgi, cocker,}    \\
                        & \tt{greyhound, retriever, brindle, hound, whippet, husky} \\

\ttbf{doughnut}         & \tt{donut, bagel} \\

\ttbf{fire hydrant}     & \tt{hydrant} \\

\ttbf{hair dryer}       & \tt{hair drier, hairdryer} \\

\ttbf{handbag}          & \tt{wallet, purse, briefcase} \\

\ttbf{horse}            & \tt{colt, pony, racehorse, stallion, equine, mare, foal, palomino, mustang, clydesdale, bronc, bronco} \\

\ttbf{ice cream}        & \tt{icecream} \\

\ttbf{knife}            & \tt{pocketknife, knive} \\

\ttbf{laptop}           & \tt{computer, notebook, netbook, lenovo, macbook} \\

\ttbf{mobile phone}     & \tt{cell phone, phone, cellphone, telephone, smartphone, iPhone} \\

\ttbf{motorcycle}       & \tt{scooter, motor bike, motor cycle, motorbike, scooter, moped} \\

\ttbf{oven}             & \tt{stovetop, stove} \\

\ttbf{person}           & \tt{kid, child, chef, baker, people, adult, rider, baby, worker, passenger, sister, biker, policeman, cop,}     \\
                        & \tt{officer, lady, cowboy, bride, groom, male, female, guy, traveler, mother, father, gentleman, pitcher,}      \\
                        & \tt{player, skier, snowboarder, skater, skateboarder, foreigner, caller, offender, coworker, trespasser,}       \\
                        & \tt{patient, politician, soldier, grandchild, serviceman, walker, drinker, doctor, bicyclist, thief, buyer,}    \\
                        & \tt{teenager, student, camper, driver, hunter, shopper, villager}                                               \\

\ttbf{plant}            & \tt{potted plant, houseplant} \\

\ttbf{refrigerator}     & \tt{fridge, freezer} \\

\ttbf{sandwich}         & \tt{burger, sub, cheeseburger, hamburger} \\

\ttbf{sheep}            & \tt{lamb, goat, ram} \\

\ttbf{stop sign}        & \tt{street sign} \\

\ttbf{suitcase}         & \tt{suit case, luggage} \\

\ttbf{teddy bear}       & \tt{teddybear} \\

\ttbf{television}       & \tt{tv, monitor} \\

\ttbf{toilet}           & \tt{urinal, commode, lavatory, potty} \\

\ttbf{traffic light}    & \tt{street light, traffic signal, stop light, streetlight, stoplight} \\

\ttbf{train}            & \tt{locomotive, tramway, caboose} \\

\ttbf{truck}            & \tt{pickup, lorry, hauler, firetruck} \\

\ttbf{van}              & \tt{minivan} \\
\bottomrule
\end{tabularx}
\end{center}
\vspace{1pt}
\small{\caption{Neural Baby Talk fine-grained class mapping list for visual words, adopted for \nocaps setting. The output vocabulary for fine-grained classification includes all of these words (object classes and corresponding fine-grained classes). This table lists 39/601 \openimages object classes, rest are added in the output vocabulary without extra fine-grained classes.
\label{table:nbt_fg}
}}
\end{table*}
